# Supplementary material for: Offsetting Unequal Competition through RL-assisted Incentive Schemes
Source: arXiv:2201.01450 source file (2022-01-05)
Supplement: Supplementary file 1 [file supp.tex]

%\appendix
%\onecolumn
%{\huge Supplementary material}
%\clearpage
%\section{Results on Market}
%\clearpage
%\input{cmaddpg}
%\input{main_maddpg}
%\input{maddpg_test}
%\clearpage
%\input{subsidy_ST}
%\input{subsidy_SA}
%\begin{multicols}{2}

%\niloy{Please elaborate the acronyms in the caption}

%\section{}
%\Cref{fig:heatmap} presents heat-maps of the strategy selection outcomes of the classifier employed in \our. The classifier of a \our\ agent trained in self-play in \ourgame\ for $150000$ episodes has been used. The positions of three other agents (two opponents and one teammate) have been kept fixed. In \cref{fig:heatmap} winning strategy corresponds to red and lossing strategy as blue. Note that, in general, classifier chooses winning strategy when at least one of the team are in advantageous position to reach the landmark quicker than any opponent.  To be more specific, \cref{fig:heatmap-5,fig:heatmap-7} show the \our\ agent selects winning strategy only for a small area surrounding the landmark, where it will play \textit{go-for-landmark} as  %either one of the \our\ team is closer to landmark than the opponents approximately.  in both of these cases, the other \our\ agent is positioned far away from the landmarks.  On the contrary, in \cref{fig:heatmap-2} one \our\ agent which is visible is closer to one landmark. Thereby, the \our\ agent, generating the heatmap, selects winning strategy over a region around the opponents, giving an impression of its planning to the role of \textit{stop-the-opponent}, handing over the role of \textit{go-for-landmark} to the other \our\ agent.

\section{Comparison with MAAC}
Here we have compared \bsln\ with MAAC in \ourgame\ with all agents having initial \texttt{max\_speed} set at 4. 
For experimentation, we have used similar hidden layer architecture as \bsln\ for fair comparison. Agents have been trained using 
the two algorithms separately for $150000$ iterations and \bsln\ team has been played against MAAC team for $1000$ test episodes. To remove possible bias in testing episodes, 500 initial configurations are generated and two episodes are played with same configuration but  the initial positions of the teams exchanged. Fig. \ref{fig:maac_vs_maddpg} shows that both algorithms perform very similar, with respect to their average team-wise landmark count. Despite the comparable performance, MAAC is very expensive to train and thereby we used \bsln\ as our underlying framework. Still the extension that we have build on \bsln\ is quite general and thereby can easily be extended over MAAC also. 
%\niloy{The result is confusing - I think better remove the reward part and just highlight the landmark part}
\begin{figure}[!ht]
	\centering
%	\subfloat[Rewards]{\includegraphics[width=0.17\textwidth]{Results/reward_4444_75000_mc-vs-md_te.pdf}}
	\subfloat[Landmark Count]{\includegraphics[width=0.17\textwidth]{Results/landmark_4444_75000_mc-vs-md_te.pdf}}
	\caption{ MAAC is compared with \bsln\ in \ourgame. Their comparable performance justifies use of computationally efficient \bsln\ in our framework. }\label{fig:maac_vs_maddpg}
\end{figure}

\section{Additional experiments on static incentive schemes}

In the main paper, we have 
reported the effects of various static schemes for a representative  set of parameters. 
Here we present a more extensive study of agents' performance and behavior under both of the static incentive schemes for a wider range of values of the corresponding parameters ($\alpha_{\tT}$ and $\alpha_{\aA}$).
To asses the agents' performance and behavior, we used the same set of metrics, namely, team-wise average reward, agent-wise average landmark count, fraction of winning policy usage and speed values.
%There, we have presented observations only for a specific value of $\alpha_{\tT}$ and $\alpha_{\aA}$. 
\Cref{fig:static-team-additional} presents results while setting $\alpha_{\tT} = 0.1, 0.3$ and $0.5$. 
%contain agents' 	performance using same measures for a wide range of values of $\alpha_{\tT}$ and $\alpha_{\aA}$ respectively. Fig. \ref{fig:static-additional} varies $\alpha_T $ for $ 0.1, 0.3, $ nd $0.5 $  and reports corresponding 
%When $\alpha_{\tT}$ gradually increase from $ 0.1 $ to $ 0.5 $, the reward plots also gradually display the improvement of the weak team with respect to the strong team. 
%With higher $\alpha_{\tT}$, the average episode reward of the teams are balanced for longer
We observe for smaller value of $\alpha_{\tT}$ strong team outperforms the weak team in reward with slowly increasing performance gap between the teams for the entire training time.
%
%We observe that for small team incentive, $\alpha_T = 0.1$ or $0.3$, the weak team reward is always outperformed by the stronger team and the performance gap is slowly increasing. 
%
Similarly in corresponding landmark count plot, we observe the weak agent is hardly improving supporting our main observation in section 3. 
While $\alpha_{\tT}$ is raised to $0.5$, the average team reward of the weak team is elevated to a point where it balances the strong team's reward for a while. But eventually as the strong team has two strong players quickly improving (as observed in the landmark count plot), the weak team's reward falls short of the other team reward. 
Despite the high team incentives, the weak agent has failed to improve its landmark reaching capability in any of these cases, as shown from the landmark counts (see column 2 in \cref{fig:static-team-additional}). 
In skill set plots, we observe in a similar way that the three agents are quickly converging to maximum speed whereas the weak agent is always finishing keeping a small gap with its competitors. Also, the rate at which the weak team takes the winning policy is increasing if we increase  the team reward, but eventually the strong team always adopts the winning policy more frequently that the weak.
From these observations, we can conclude that however large the team incentive is, it is unable to balance both team reward in a long run and eventually strong team outperforms the weak team.
\begin{figure*}[!ht]
	\centering
	\subfloat[Rewards]{\includegraphics[width=0.17\textwidth]{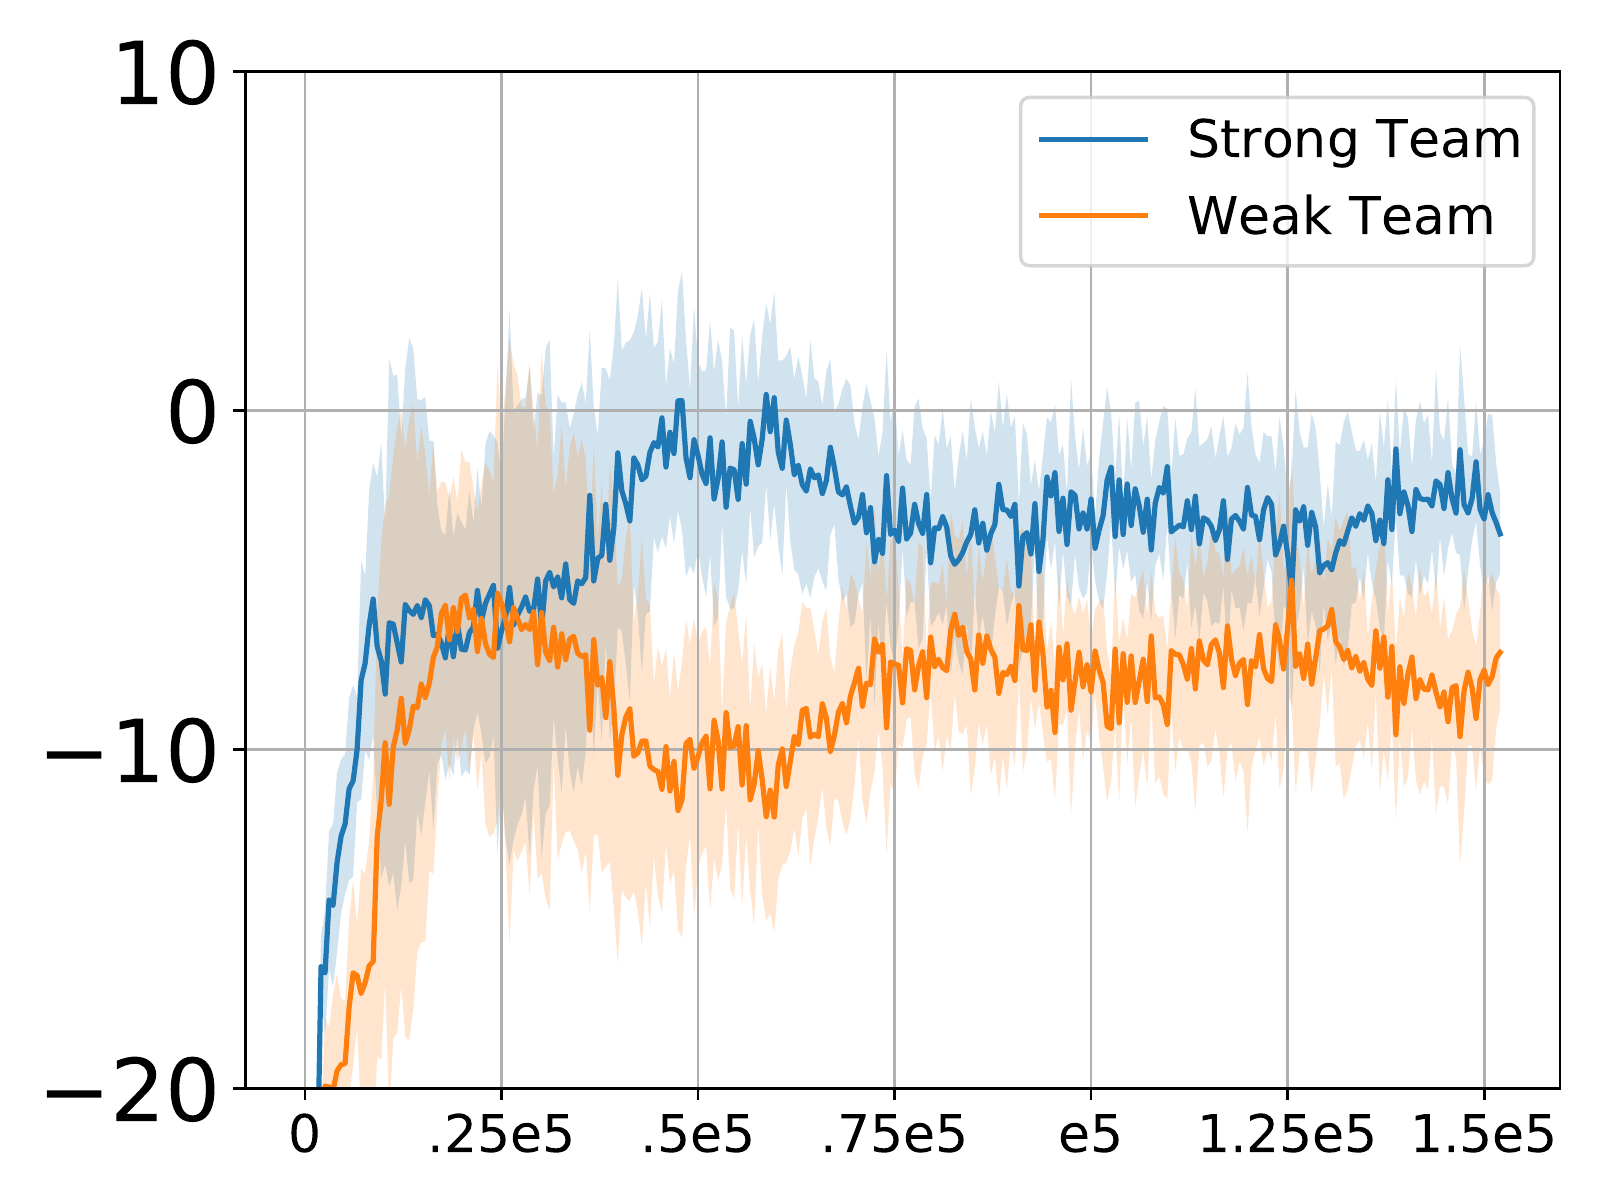}}
	\subfloat[Landmark]{\includegraphics[width=0.17\textwidth]{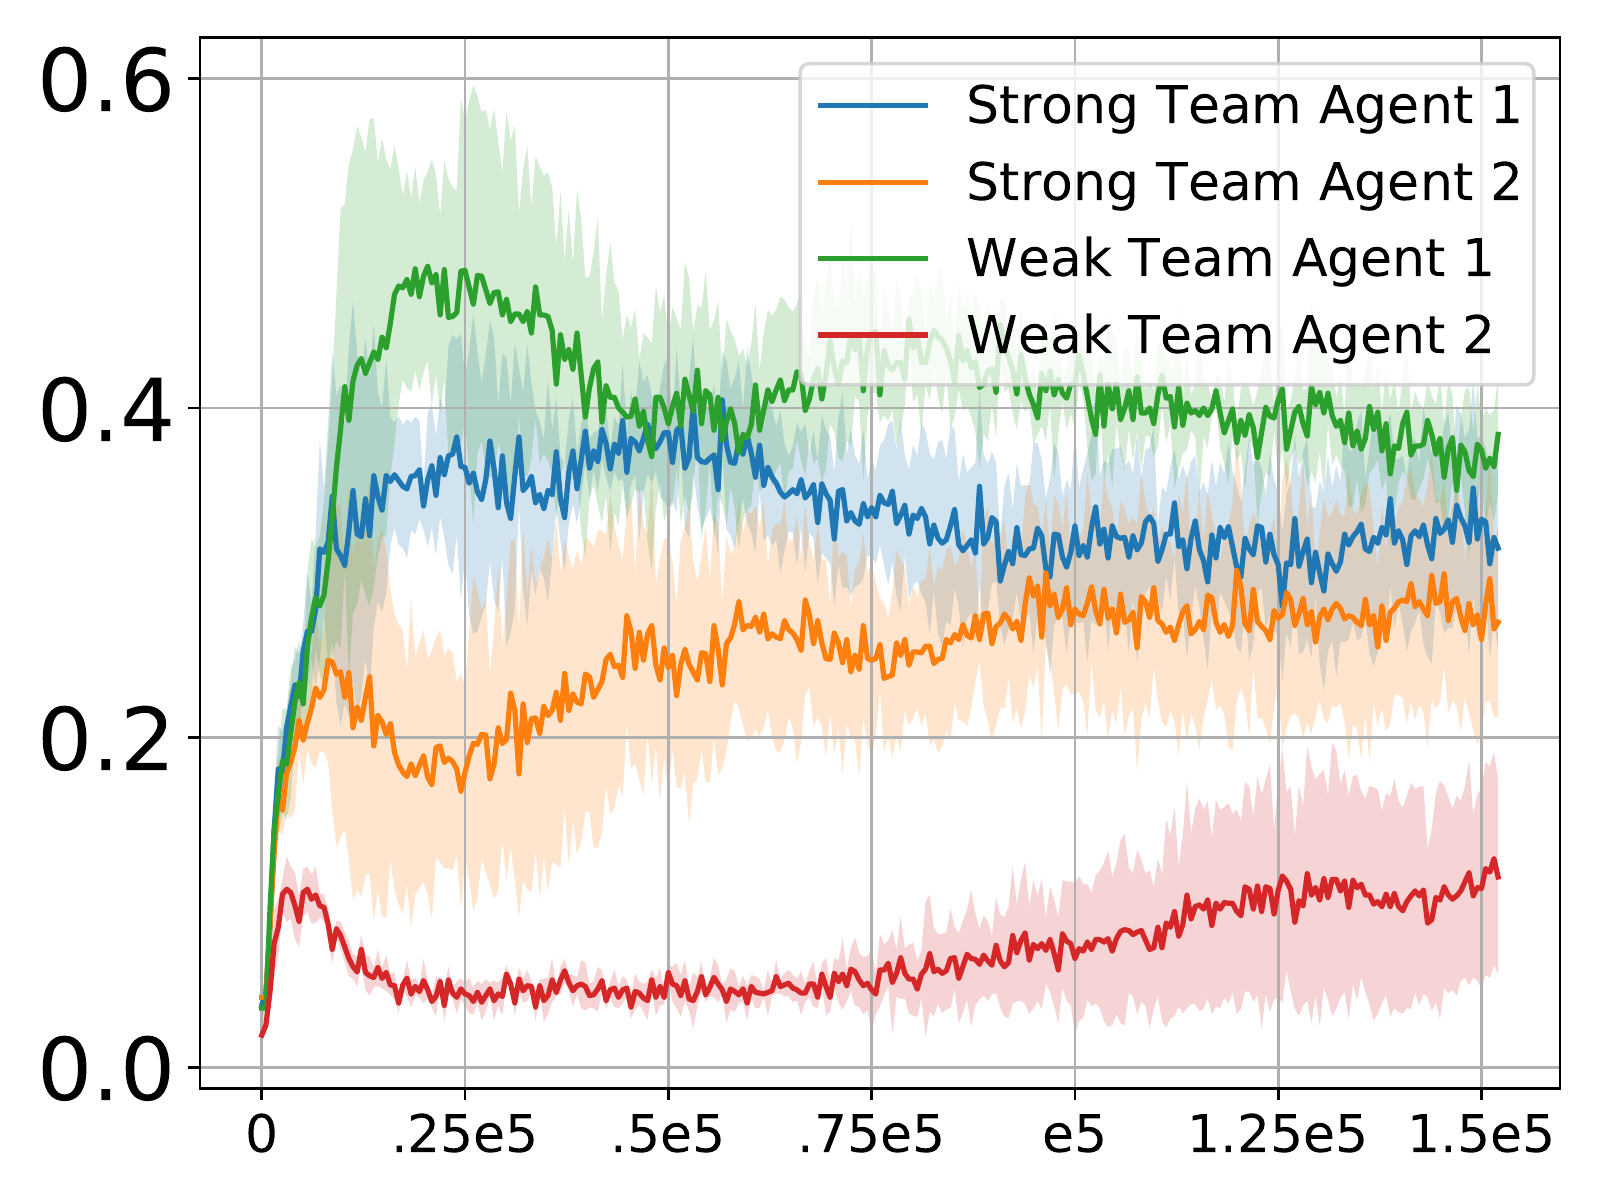}}
	\subfloat[Win Policy Usage]{\includegraphics[width=0.17\textwidth]{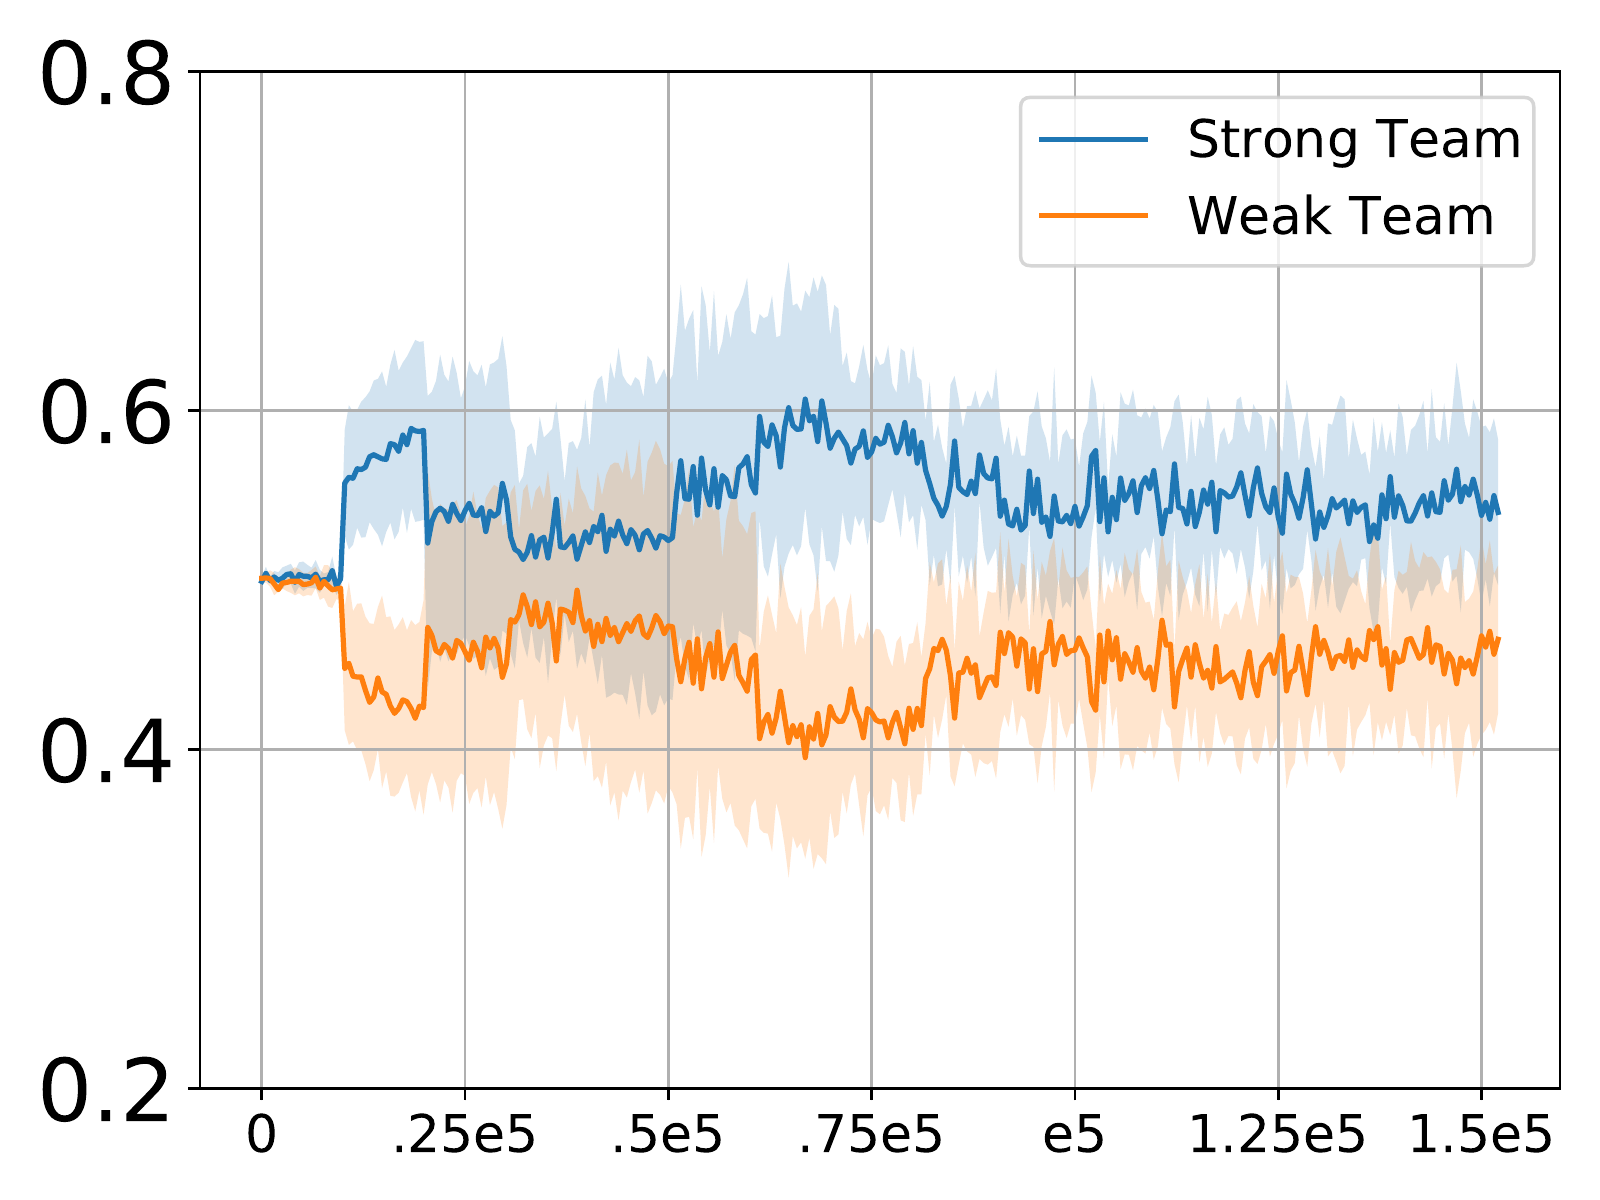}}
	\subfloat[Speed]{\includegraphics[width=0.17\textwidth]{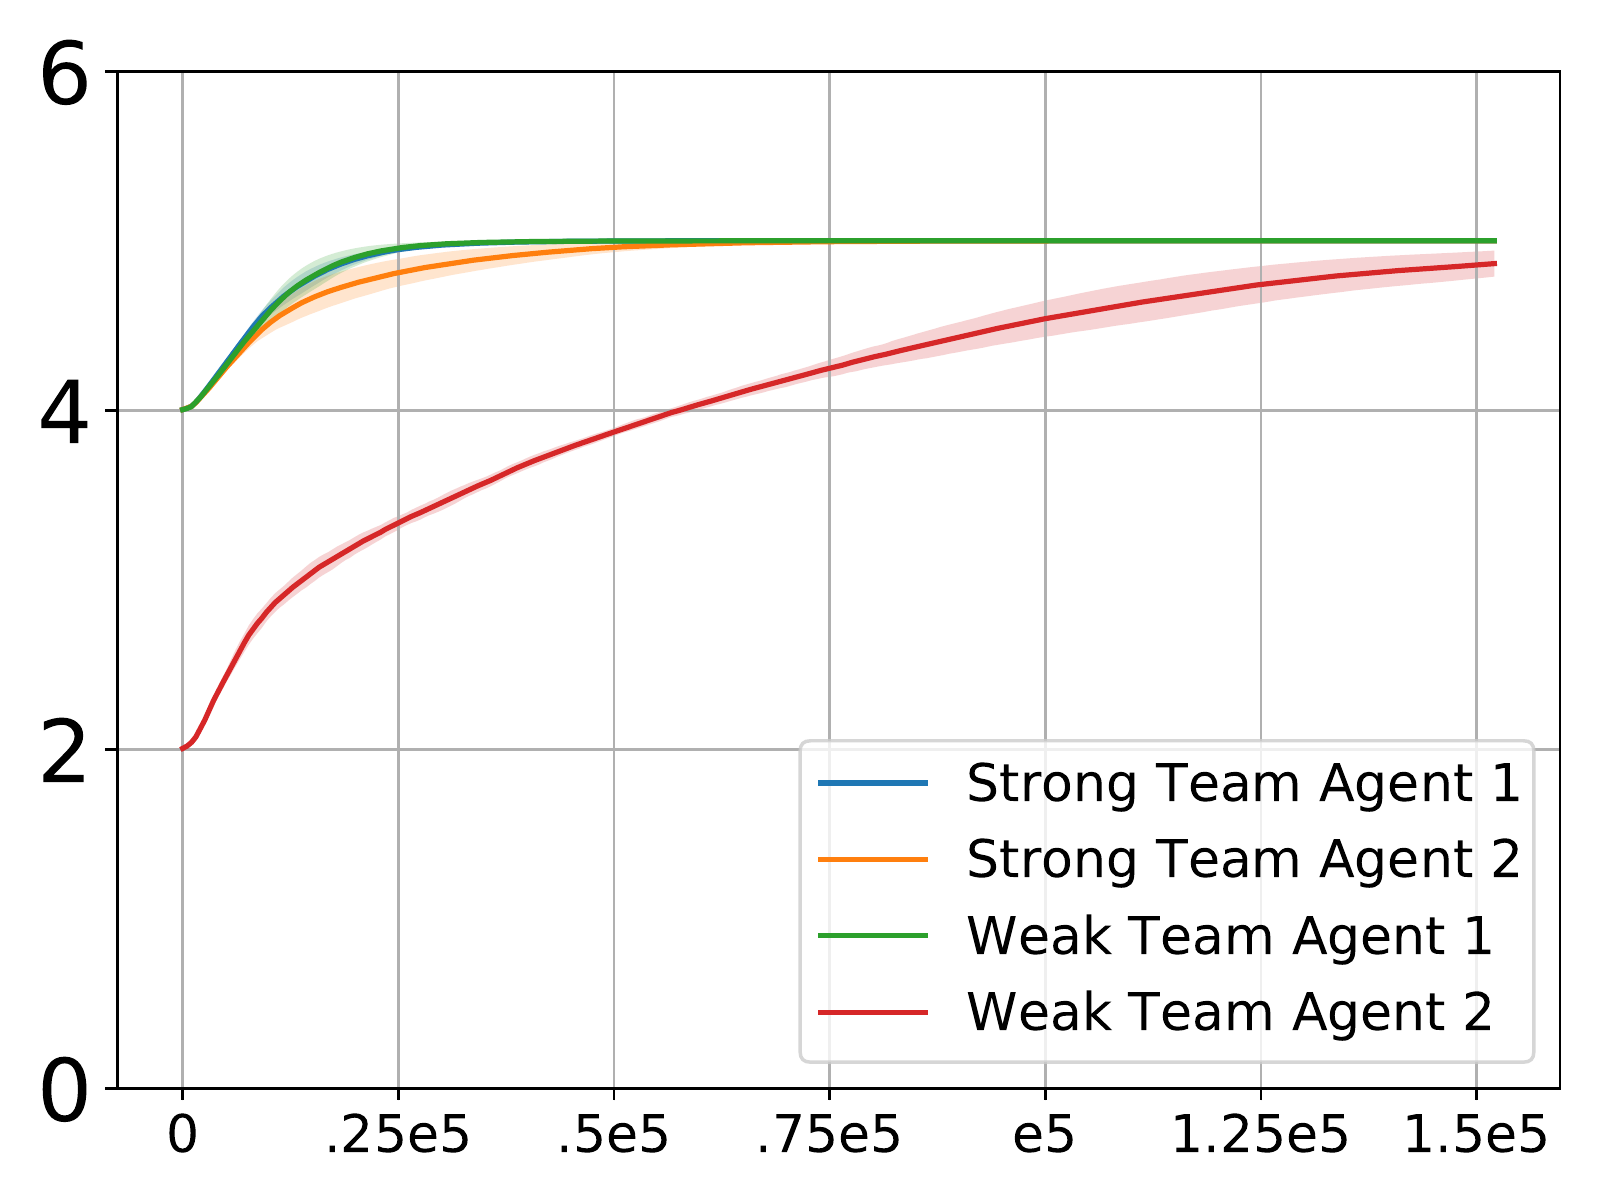}}
	\\
	\subfloat[Rewards]{\includegraphics[width=0.17\textwidth]{Results/ag_rewards_StaticTeam_30_mean_classify_tr.pdf}}
	\subfloat[Landmark]{\includegraphics[width=0.17\textwidth]{Results/landmark_StaticTeam_30_mean_classify_tr.pdf}}
	\subfloat[Win Policy Usage]{\includegraphics[width=0.17\textwidth]{Results/win-policy-stat_StaticTeam_30_mean_classify_tr.pdf}}
	\subfloat[Speed]{\includegraphics[width=0.17\textwidth]{Results/speed_StaticTeam_30_mean_classify_tr.pdf}}
	\\
	\subfloat[Rewards]{\includegraphics[width=0.17\textwidth]{Results/ag_rewards_StaticTeam_50_mean_classify_tr.pdf}}
	\subfloat[Landmark]{\includegraphics[width=0.17\textwidth]{Results/landmark_StaticTeam_50_mean_classify_tr.pdf}}
	\subfloat[Win Policy Usage]{\includegraphics[width=0.17\textwidth]{Results/win-policy-stat_StaticTeam_50_mean_classify_tr.pdf}}
	\subfloat[Speed]{\includegraphics[width=0.17\textwidth]{Results/speed_StaticTeam_50_mean_classify_tr.pdf}}
	\\
	\caption{ Agents trained for \ourgame\ using \our\ under static team-wise incentives for $\alpha_{\tT} = 0.1, 0.3$ and $0.5$ respectively. The results indicate even larger $\alpha_{\tT}$ can not improve the weaker agent, in effect failing to balance the outcome of the teams. 
		\label{fig:static-team-additional}	
	}
\vspace{-3mm}
\end{figure*}

\begin{figure*}[!ht]
	\centering
	\subfloat[Rewards]{\includegraphics[width=0.17\textwidth]{Results/ag_rewards_StaticAgent_3030_mean_classify_tr.pdf}}
	\subfloat[Landmark]{\includegraphics[width=0.17\textwidth]{Results/landmark_StaticAgent_3030_mean_classify_tr.pdf}}
	\subfloat[Win Policy Usage]{\includegraphics[width=0.17\textwidth]{Results/win-policy-stat_StaticAgent_3030_mean_classify_tr.pdf}}
	\subfloat[Speed]{\includegraphics[width=0.17\textwidth]{Results/speed_StaticAgent_3030_mean_classify_tr.pdf}}
	\\
	\subfloat[Rewards]{\includegraphics[width=0.17\textwidth]{Results/ag_rewards_StaticAgent_3050_mean_classify_tr.pdf}}
	\subfloat[Landmark]{\includegraphics[width=0.17\textwidth]{Results/landmark_StaticAgent_3050_mean_classify_tr.pdf}}
	\subfloat[Win Policy Usage]{\includegraphics[width=0.17\textwidth]{Results/win-policy-stat_StaticAgent_3050_mean_classify_tr.pdf}}
	\subfloat[Speed]{\includegraphics[width=0.17\textwidth]{Results/speed_StaticAgent_3050_mean_classify_tr.pdf}}
	\\
	\subfloat[Rewards]{\includegraphics[width=0.17\textwidth]{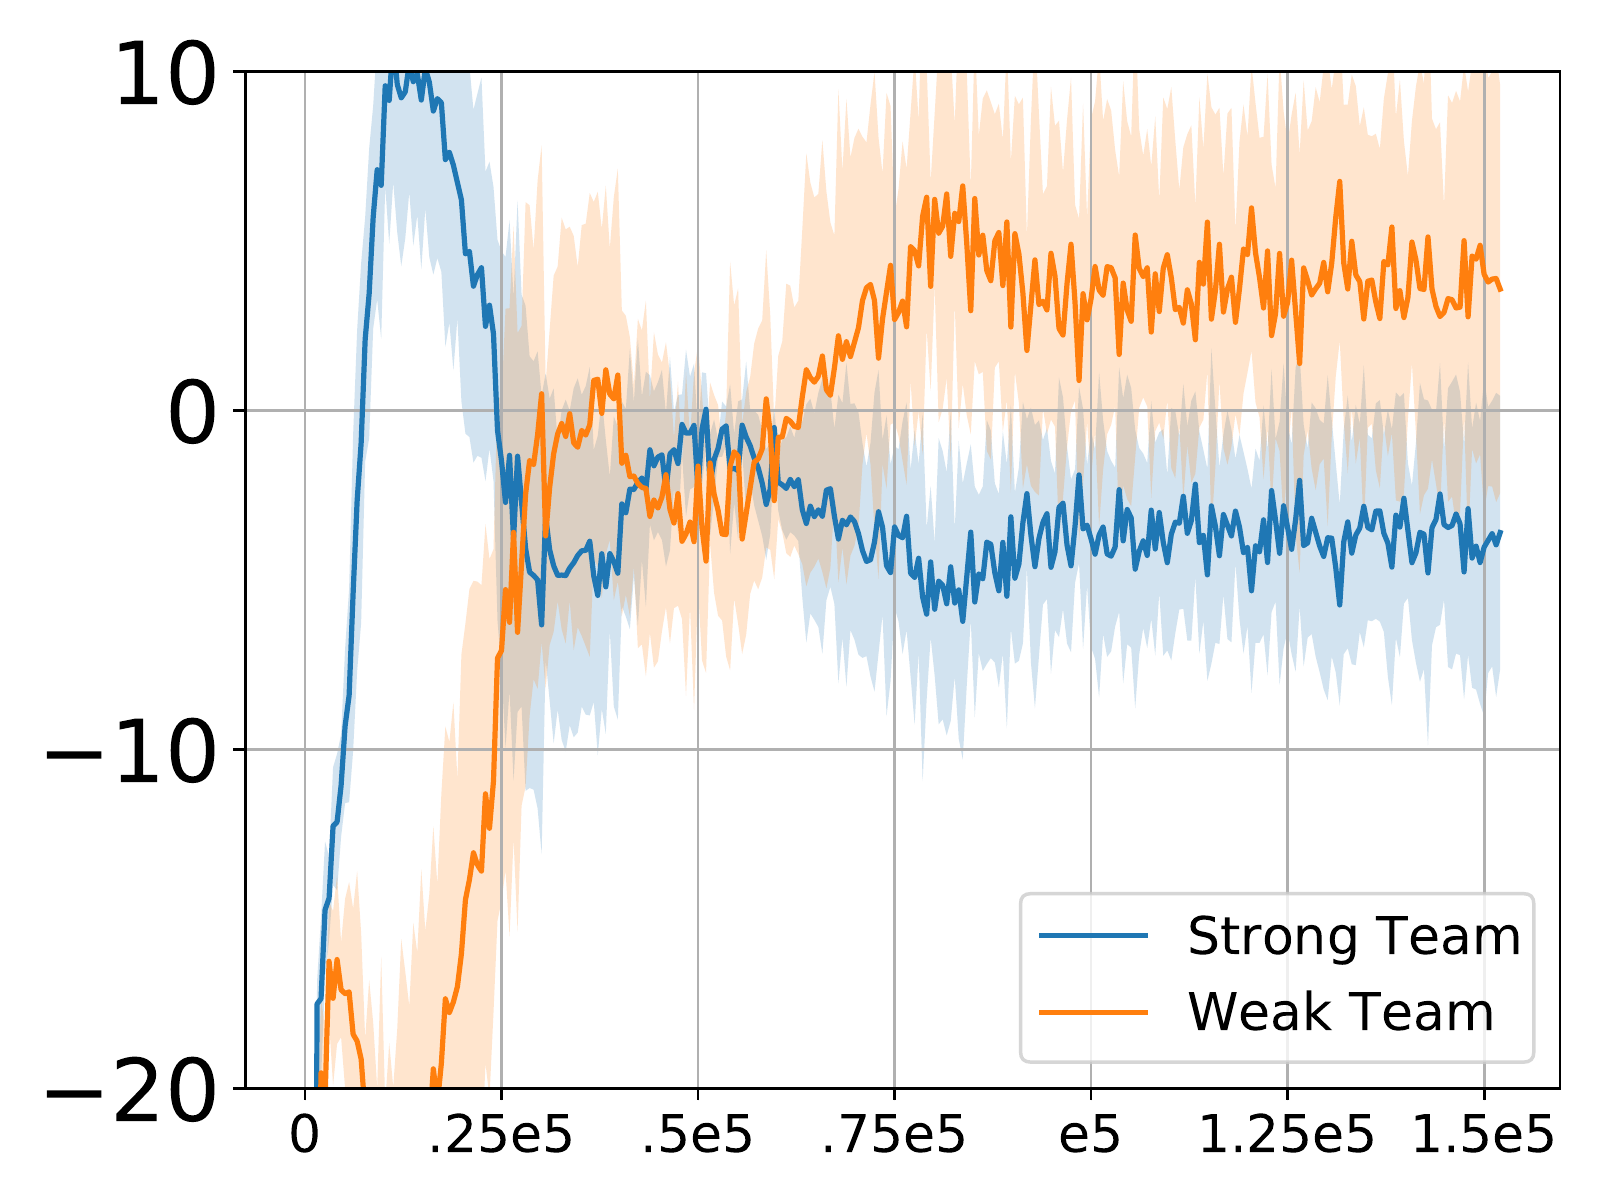}}
	\subfloat[Landmark]{\includegraphics[width=0.17\textwidth]{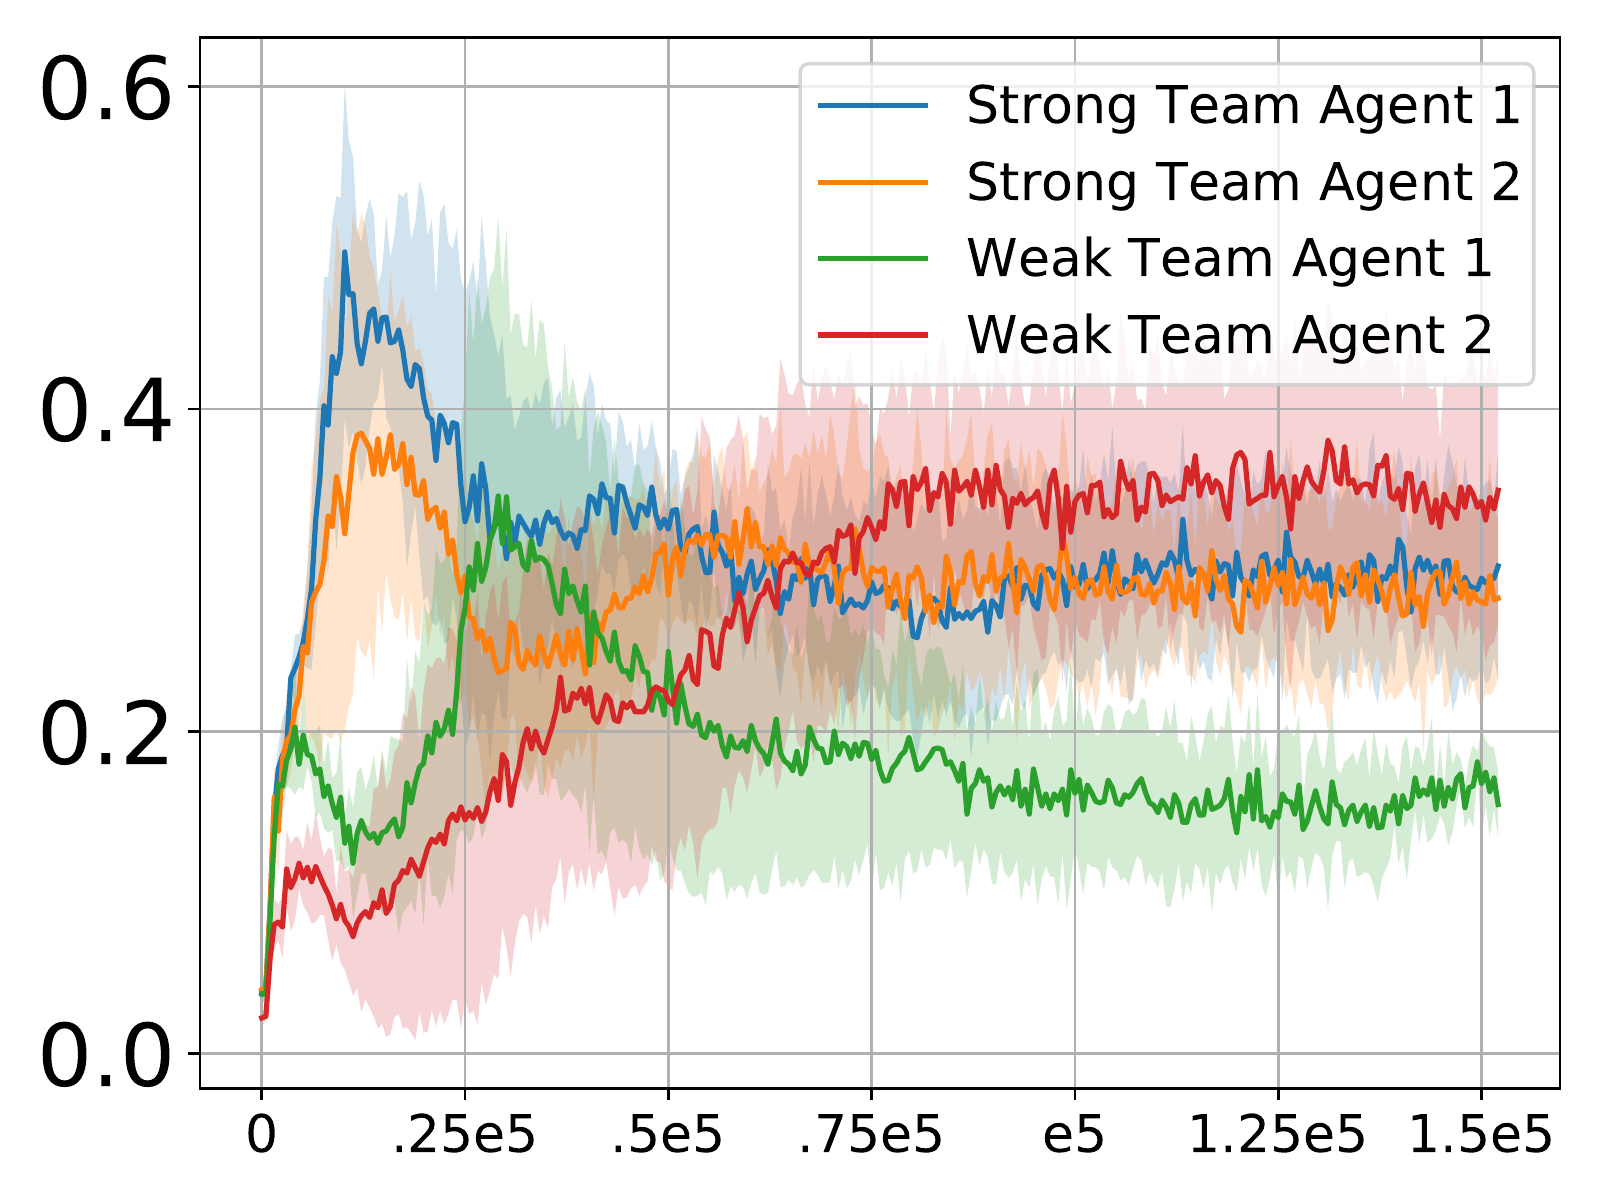}}
	\subfloat[Win Policy Usage]{\includegraphics[width=0.17\textwidth]{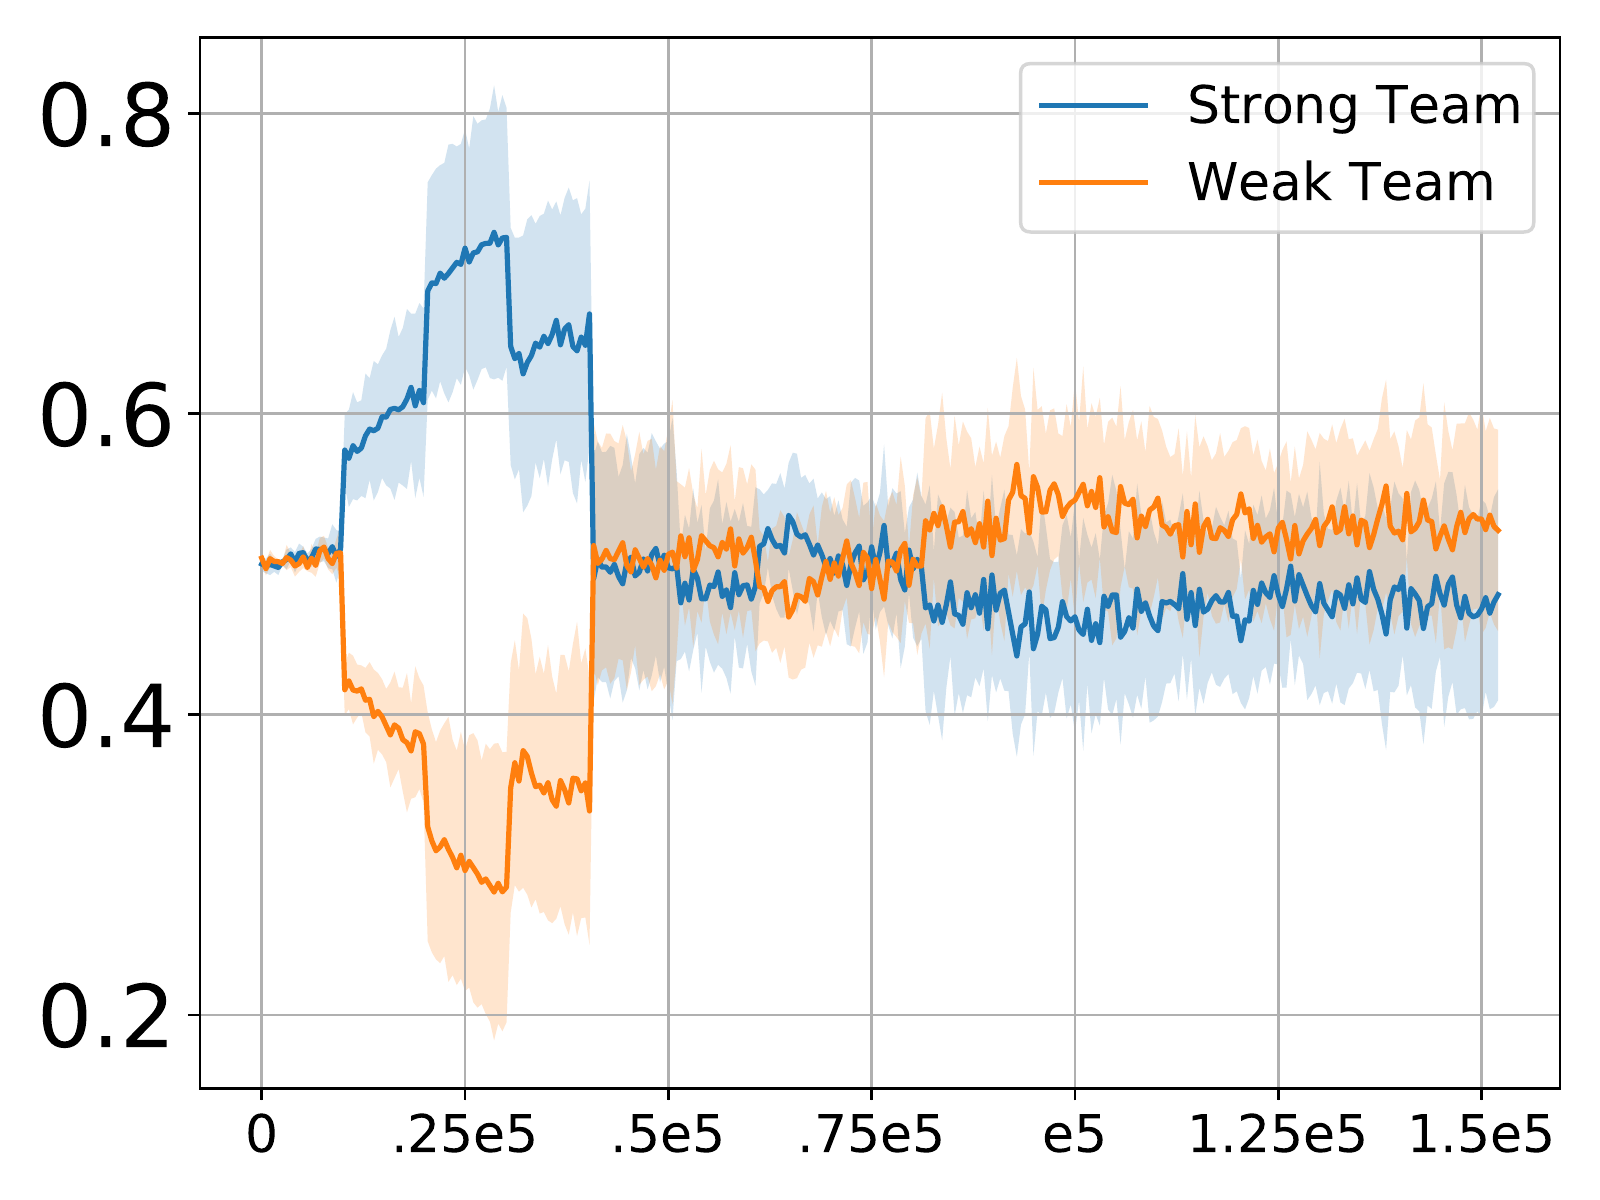}}
	\subfloat[Speed]{\includegraphics[width=0.17\textwidth]{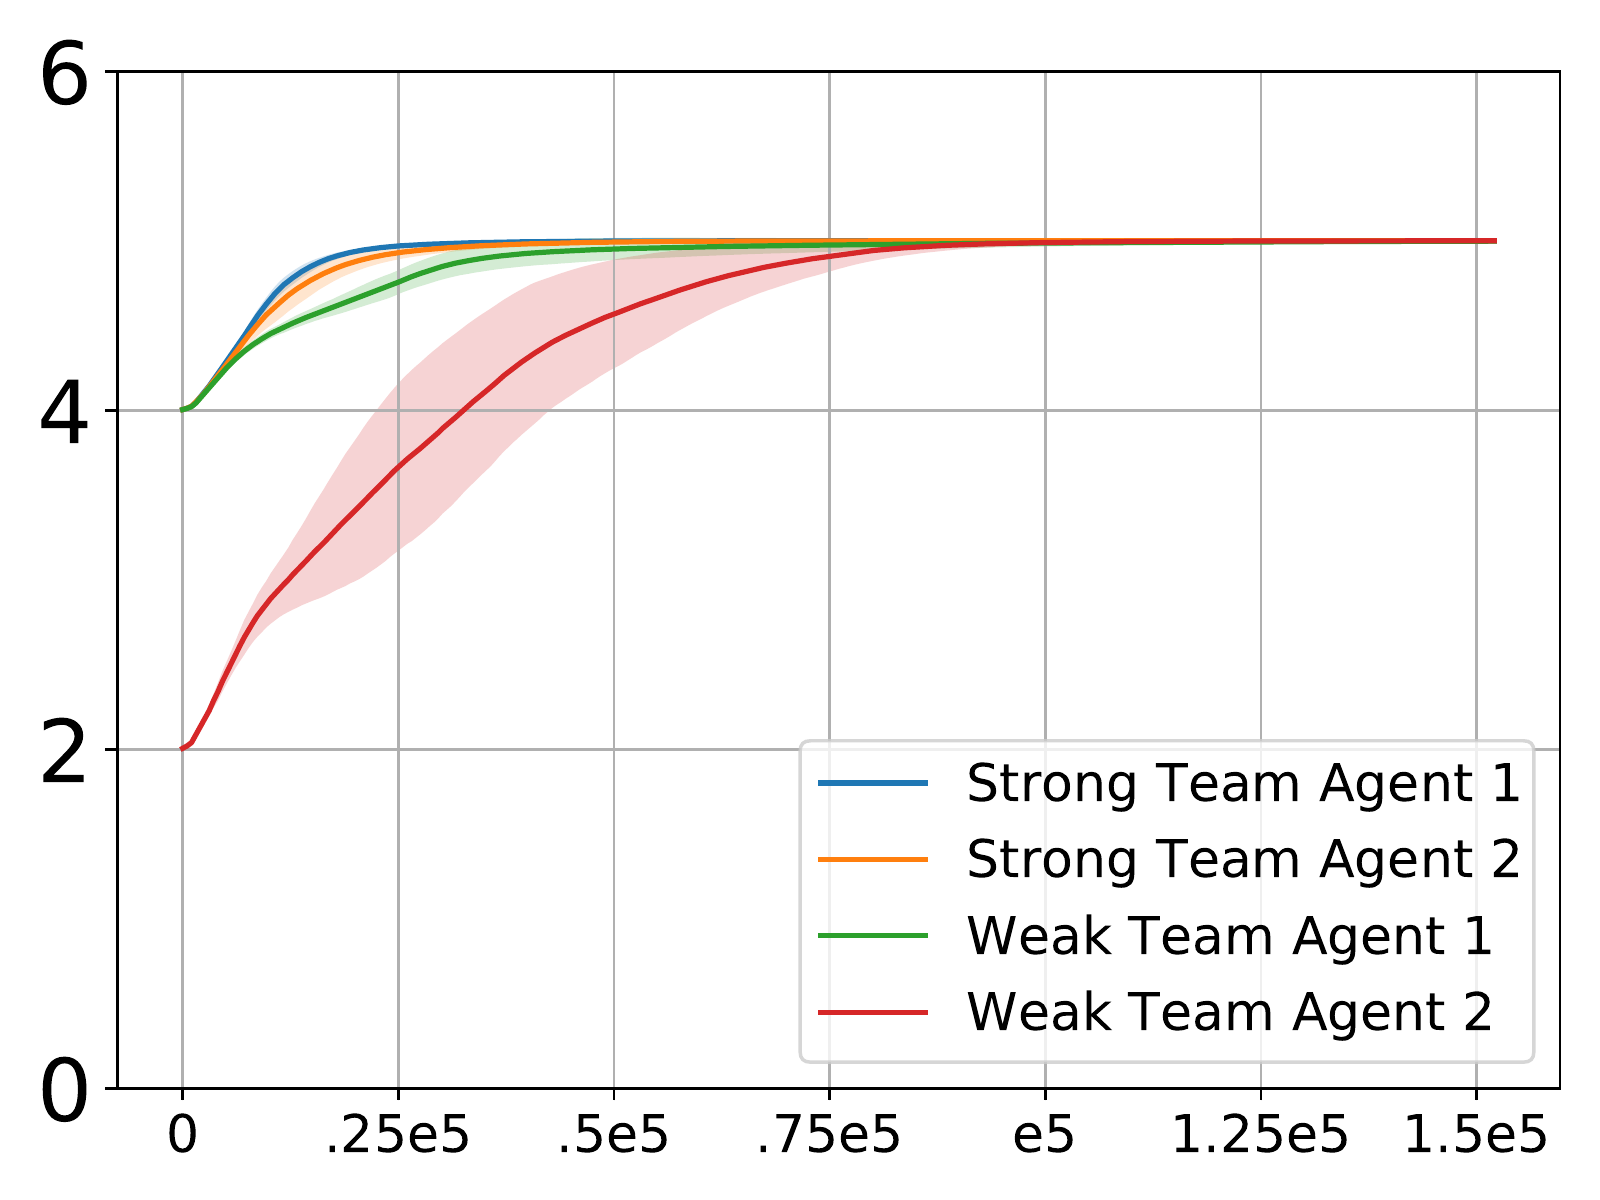}}
	\\
	\caption{ Agents trained for \ourgame\ using \our\ under static agent-wise incentives for $\alpha_{\aA} = 0.3, 0.5$ and $0.7$ respectively. Results indicate agent-wise incentive becomes redundant after balancing both team rewards for a while for all values of $\alpha_{\aA}$. }\label{fig:static-agent-additional}
\end{figure*}

% The landmark plot is justiarious fying the inferior performance of the weak team throughout by revealing that 

%Even for a very high value of $\alpha_T $, $\alpha_T = 0.9$ we observe the balance of the two team reward is maintained for longer, but very slowly the strong team has started to outperform the weak team. In the landmark
Further we explore the effects of static agent-wise incentives for various configurations of $\alpha_{\aA}$. We fix team incentive to $\alpha_T= 0.3$ and vary $\alpha_{\aA}$ from $ 0.3 $ to $ 0.7 $. When $\alpha_{\aA}$ is set to $ 0.3 $, 
%we observe it has failed to make any significant changes in the final reward of the teams and thereby the weak team keeps a large reward gap from the other team. 
we observe, the weak team outperforms the strong team with a small margin. As $\alpha_{\aA}$ is raised to $0.5$ or $0.7$, the margin increases and the weak team surpasses the reward of strong team faster. 
In all the cases, we notice considerable improvement in the weak agents' landmark count performance. Also we observe, higher $\alpha_{\aA}$ results in better performance of the weak agent.
The landmark plot indicates as soon as the weak team discovers the large reward for the weak agent, touching the landmark, the team starts giving the weak player chances to touch the landmark, which results in improving performance of the weak agent to a point where the weak team is comparable with the strong team. 
The speed of the weak agent also improves to the speed of the other agents, unlike the gap in team-wise incentives. Similarly, the weak team starts to take the winning policy more frequently than the strong team. 
But as we already indicated, once the weak team improves to the level of the strong team,
% and starts  performing as well
 the extra agent incentive becomes inessential and needs to be adjusted accordingly. The static incentive scheme has no scope to 
adjust, resulting in the weak team outperforming the strong team in total rewards by leveraging the undue advantage of the extra agent incentive. 
%We observe this trend for $\alpha_{\aA}$ in all the cases, although the exact point where the weak team reward exceeds the strong team reward, differs in these cases. 

\if{0}

\section{Additional Experiments of Dynamic Incentive Schemes with RL Agents}
In section $4$, we have introduced dynamic incentive schemes enriched with a RL agent. The RL agent takes as input the speeds of the agents and try to infer appropriate mapping between speed and landmark information to deliver correct incentives. 

Here we have experimented with a modified version of both Team-RL-Agent-Dynamic and Team-Dynamic-Agent-RL incentive schemes where the RL agent takes as input both the speed of all the agents and policy of only the weak team. 

\textbf{Team-RL-Agent-Dynamic-With-Policy} Here the agent incentive is decided using eq. ($4$) and team incentive $\alpha_{\tT}$ is decided by sampling from $\pi(s,\phi(\pi_{weak}))$ where $\phi( \pi_{weak} )$ is a manually designed feature representation of the policies of the weak team $\pi_{weak}$ and $s$ denotes the speed configurations of all agents.

\textbf{Team-Dynamic-Agent-RL-With-Policy} Here the team incentive $\alpha_{\tT}$ is decided using eq. ($4$) and agent incentive $\alpha_{\aA}$ is decided by sampling from $\pi(s,\phi(\pi_{weak}))$ where $\phi( \pi_{weak} )$ is a manually designed feature representation of the policies of the weak team $\pi_{weak}$ and $s$ denotes the speed configurations of all agents.

Fig \ref{fig:team-rl-agent-dyn} illustrates the results for \textbf{Team-RL-Agent-Dynamic-With-Policy}. We observe that after balancing the rewards of the teams for a while the strong team slowly starts to outperform the weak team. This behavior resembles the static team wise incentive scheme. Also \cref{fig:team-rl-agent-dyn-count} reveals the weak agent has not been able to learn the policy much, neither has it improved its speed \cref{fig:team-rl-agent-dyn-speed}. Therefore, almost in the same way as static team-wise reward, the presence of the weak agent, who could not improve, hinders the improvement of the team, limiting its reward or winning policy usage \cref{fig:team-rl-agent-dyn-win-policy-stat}. Fig. \ref{fig:team-rl-agent-dyn-subsidy} reveals the reason where we find the fast increment of the speed of the weak agent forces $\alpha_{\aA}$ to diminish too fast before the weak agent can improve, and we have already observed in static team incentive schemes that without sufficient agent incentive the weak team can not compete in long run. Also the randomness in the team incentive $\alpha_{\tT}$ reveals expanding the observation space has adversely affected the learning as larger observation space requires even more samples which are very expensive in our case. So we can conclude obtaining $\alpha_{\aA}$ only from speed will always be inefficient for improving the weak team upto the level of the strong team. Moreover in our  setting, where samples are expensive, expanding observation does not help, rather inversely affect the learning. 
\begin{figure}[!t]
	\centering
	\subfloat[ag rewards]{\includegraphics[width=0.17\textwidth]{Results/ag_rewards_team-rl-ag-dyn_1_classify_rl_tr.pdf}}\label{fig:team-rl-agent-dyn-score}
	\subfloat[landmark]{\includegraphics[width=0.17\textwidth]{Results/landmark_team-rl-ag-dyn_1_classify_rl_tr.pdf}}\label{fig:team-rl-agent-dyn-count}
	\subfloat[win-policy-stat]{\includegraphics[width=0.17\textwidth]{Results/win-policy-stat_team-rl-ag-dyn_1_classify_rl_tr.pdf}}\label{fig:team-rl-agent-dyn-win-policy-stat}
	\subfloat[speed]{\includegraphics[width=0.17\textwidth]{Results/speed_team-rl-ag-dyn_1_classify_rl_tr.pdf}}\label{fig:team-rl-agent-dyn-speed}
	\subfloat[subsidy]{\includegraphics[width=0.17\textwidth]{Results/subsidy_team-rl-ag-dyn_1_classify_rl_tr.pdf}}\label{fig:team-rl-agent-dyn-subsidy}
	\caption{ Team-RL-Agent-Dynamic-Incentive scheme where Team wise reward is obtained from an RL scheme taking both speed and policy and Agent wise reward is obtained from their
		difference in speed}\label{fig:team-rl-agent-dyn}
\end{figure}

Fig \ref{fig:team-dyn-agent-rl} illustrates the results for \textbf{Team-Dynamic-Agent-RL-With-Policy}. We observe the rewards of the teams are roughly balanced \cref{fig:team-rl-agent-dyn-score}, the speeds are converging \cref{fig:team-rl-agent-dyn-speed} and winning policy is taken by both teams in equivalent frequency \cref{fig:team-rl-agent-dyn-win-policy-stat}. Moreover, in \cref{fig:team-rl-agent-dyn-count} shows each agent has an equivalent performing agent in the other team, balancing their performance. So, employing RL agent for agent-wise incentive helps the system to learn a better mapping from speed to incentive to provide sufficient support to the weak agent to sustain and grow.  So, we can conclude if we can use RL agent only for one component of the incentive, it is more judicious to use that for the agent-wise incentive.
The downside of this scheme is two-fold, first, the randomness and second the static behavior of $\alpha_{\aA}$, the reason for both lying in the fact that the expanded observation space has increased the sample requirement which is difficult to meet in our cases where samples are expensive. Therefore despite choosing an appropriate $\alpha_{\aA}$ initially, the RL agent fails to reduce the $\alpha_{\aA}$ when weak team improves, resulting in high rewards for weak team, a problem similar to static agent wise incentive. 

In summary we can conclude, it is always judicious to employ RL agent for $\alpha_{\aA}$ instead of $\alpha_{\tT}$ and considering the adverse effects of higher sample complexity for including the policy information, we should keep the observation space confined to speed configurations only.

\begin{figure}[!t]
	\centering
	\subfloat[ag rewards]{\includegraphics[width=0.17\textwidth]{Results/ag_rewards_team-dyn-ag-rl_2_classify_rl_tr.pdf}}\label{fig:team-dyn-agent-rl-score}
	\subfloat[landmark]{\includegraphics[width=0.17\textwidth]{Results/landmark_team-dyn-ag-rl_2_classify_rl_tr.pdf}}\label{fig:team-dyn-agent-rl-count}
	\subfloat[win-policy-stat]{\includegraphics[width=0.17\textwidth]{Results/win-policy-stat_team-dyn-ag-rl_2_classify_rl_tr.pdf}}\label{fig:team-dyn-agent-rl-win-policy-stat}
	\subfloat[speed]{\includegraphics[width=0.17\textwidth]{Results/speed_team-dyn-ag-rl_2_classify_rl_tr.pdf}}\label{fig:team-dyn-agent-rl-speed}
	\subfloat[subsidy]{\includegraphics[width=0.17\textwidth]{Results/subsidy_team-dyn-ag-rl_2_classify_rl_tr.pdf}}\label{fig:team-dyn-agent-rl-subsidy}
	\caption{Team-Dynamic-Agent-RL-Incentive scheme where Agent wise reward is obtained from an RL scheme taking both speed and policy and Team wise reward is obtained from their difference in speed}\label{fig:team-dyn-agent-rl}
\end{figure}

\fi
