# Supplementary material for: Offsetting Unequal Competition through RL-assisted Incentive Schemes
Source: arXiv:2201.01450 source file (2022-01-05)
Supplement: Supplementary file 2 [file 070appendix.tex]

add
